# Supplementary material for: Investigating finite-size effects in molecular dynamics simulations of ion diffusion, heat transport, and thermal motion in superionic materials
Source: arXiv:2203.09558 ancillary file (2022-03-17)
Supplement: Supplementary file 1 [file Supp_Info.pdf]

Supplementary Material to
# "Investigating finite-size effects in molecular dynamics simulations of ion diffusion, heat transport, and thermal motion in superionic materials"

Federico Grasselli[1]

[1]*COSMO – Laboratory of Computational Science and Modelling, IMX, École Polytechnique Fédérale de Lausanne, 1015 Lausanne, Switzerland*

## S1. HEAT CAPACITY

The isochoric molar specific heat capacity is obtained from the finite-difference derivative of the average energy with respect to the temperature:

$$c_V = \frac{\nu \mathcal{N}_A}{N} \frac{\partial \langle E \rangle_{NVT}}{\partial T}. \tag{S1}$$

In this equation, $\langle E \rangle_{NVT}$ is the mean energy in the $NVT$ ensemble, $\nu$ is the number of atoms per formula unit, and $\mathcal{N}_A$ is the Avogadro number. I checked that these values are consistent with calculations obtained from the variance of the energy in $NVT$ simulations:

$$c_V = \frac{\nu \mathcal{N}_A}{N} \frac{\langle E^2 \rangle_{NVT} - \langle E \rangle_{NVT}^2}{kT^2}, \tag{S2}$$

where $k$ is Boltzmann's constant. The comparison between Eqs. (S1) and (S2) is shown in Fig. S1, for the case of $CaF_2$. The values and their uncertainty are estimated via a block analysis (with reshuffling to further decorrelate elements of each block). One structure every 25 MD steps was retained, to avoid having strongly correlated structures in the sampling. Details can be found in the Python Jupyter Notebook in the Materials Cloud Repository of this work. For the uncertainty on $c_V$ extracted from finite differences, I propagate the block-analysis uncertainty on the temperature-dependent mean energy, $\langle E \rangle_{NVT}$, assuming independence between values at different temperatures. The values are compatible within their error bars. The positions of the maxima, which are interpreted as the size-dependent critical temperatures to the superionic phase, are compatible as well.

Since the uncertainty on $\langle E \rangle$ goes like $\sqrt{N}$, the uncertainty on the *specific* heat capacity $c_V$ obtained from finite differences goes like $1/\sqrt{N}$. Instead, the standard deviation on the sample variance is proportional to the sample variance itself: this means that the uncertainty on var$(E)$ goes like $N$, and the uncertainty on the *specific* heat capacity from the variance formula is *independent of* $N$, and, in the performed simulations, smaller than that obtained from finite differences. This is evident in Fig. S1. Nonetheless, I decided to use the finite-difference formula in the results displayed in Fig. 2 of the main text, since the estimate is more stable near phase transitions.

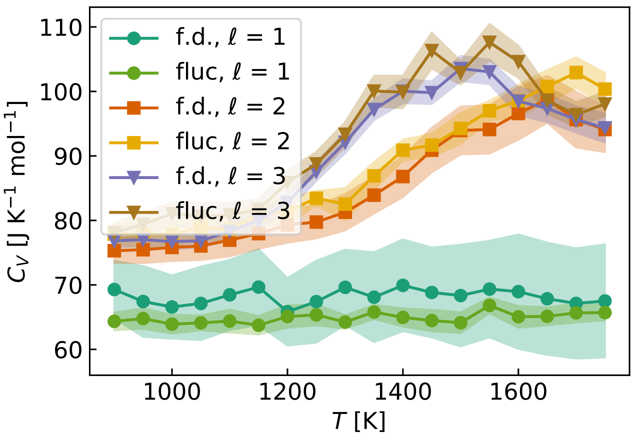


FIG. S1. Comparison between the finite-difference, Eq. (S1), and the variance methods, Eq. (S2), in the calculation of the specific heat capacity of $CaF_2$ at different temperatures.

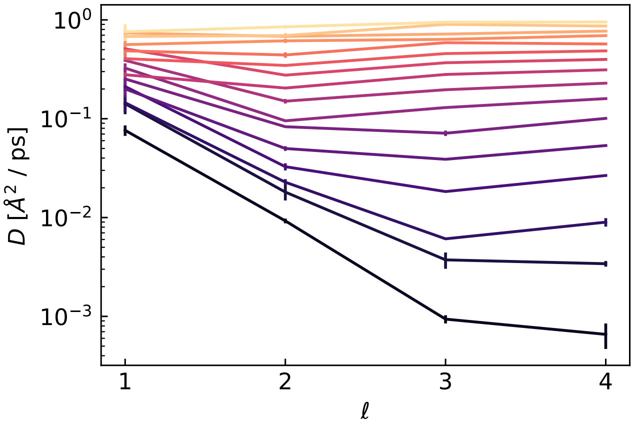


FIG. S2. System size dependence of the diffusivity of fluorine ions in $PbF_2$. Lines connect simulations at the same temperature $T$, from 500 K (black) to 1250 K (orange) every 50 K.

## S2. DIFFUSION COEFFICIENT

In this Section I report additional information on the study of the diffusion coefficient of the mobile species. Notice that, in the main manuscript, I employ the temperature $T$ as the abscissa, reporting the results at different sizes as different data sets on the same plot. In fact, such representation highlights *1)* the shift of the SI

transition temperature with system size, and *2)* the size dependence of the activation energy (the slope in the Arrhenius plot). These features would not be clear in a plot, like Fig. S2, having as abscissa the system size.

### A. Reference frames and diffusivity

For a given species $S$, I dub $D_S^{self}$ its *self*-diffusion coefficient, i.e. the diffusivity computed in the reference frame where its centre of mass is fixed. Here I show that it is immediate to relate $D_S^{self}$ to the diffusivity $D_S$ computed in the *barycentric* reference frame, where the total c.m. is fixed, as it is customary in equilibrium MD simulations. In fact, by employing the Green-Kubo formula for the diffusivity,

$$\begin{aligned} D_S^{self} &= \frac{1}{N_S}\sum_{i=1}^{N_S}\int_0^\infty \langle [\mathbf{v}_i^S(t) - \mathbf{V}^S(t)]\cdot \\ &[\mathbf{v}_i^S(0) - \mathbf{V}^S(0)]\rangle\, dt \\ &= \frac{1}{N_S}\sum_{i=1}^{N_S}\int_0^\infty \langle \mathbf{v}_i^S(t)\cdot \mathbf{v}_i^S(0)\rangle dt \\ &- 2\frac{1}{N_S}\sum_{i=1}^{N_S}\int_0^\infty \langle \mathbf{v}_i^S(t)\cdot \mathbf{V}^S(0)\rangle dt \\ &+ \frac{1}{N_S}\sum_{i=1}^{N_S}\int_0^\infty \langle \mathbf{V}^S(t)\cdot \mathbf{V}^S(0)\rangle dt \end{aligned} \tag{S3}$$

where $\mathbf{v}_i^S(t)$ is the velocity of the $i$-th atom of species $S$, and $\mathbf{V}^S(t) \equiv \frac{1}{N_S}\sum_{i=1}^{N_S}\mathbf{v}_i^S(t)$. Therefore,

$$\begin{aligned} D_S^{self} &= \frac{1}{N_S}\sum_{i=1}^{N_S}\int_0^\infty \langle \mathbf{v}_i^S(t)\cdot \mathbf{v}_i^S(0)\rangle dt \\ &- \int_0^\infty \langle \mathbf{V}^S(t)\cdot \mathbf{V}^S(0)\rangle dt \\ &= D_S - \mathcal{D}_S, \end{aligned} \tag{S4}$$

where the last term at RHS, $\mathcal{D}_S$, is the diffusivity of the c.m. of the species $S$ in the barycentric reference frame. Moreover, in a system (like the SI phases of the materials inspected in this work) where there is a solid matrix of non-diffusive atoms of mass $m'$ (primed quantities), and a diffusive species of mobile atoms of mass $m$ (non-primed quantities), it is often useful to express the diffusivity of the latter in the *laboratory* reference frame, where the solid matrix is fixed. Since, for a simulation performed in the barycentric reference frame,

$$\mathbf{V}' = -\frac{N_d}{N'}\frac{m}{m'}\mathbf{V}, \tag{S5}$$

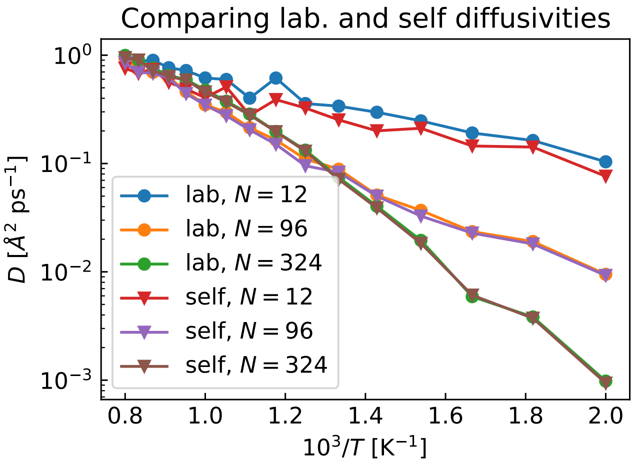


FIG. S3. Arrhenius plots for the diffusivity of $PbF_2$ computed in the laboratory reference frame (where the total momentum of the matrix of Pb ions vanishes) and in the reference frame where the total momentum of the diffusing F ions vanishes (self-diffusivity). Significant differences are only seen at very small size.

the diffusivity of the diffusive species in the laboratory frame can be expressed as

$$\begin{aligned} D_d^{lab} &\equiv \frac{1}{N_d}\sum_{i=1}^{N_d}\int_0^\infty \langle [\mathbf{v}_i(t) - \mathbf{V}'(t)]\cdot[\mathbf{v}_i(0) - \mathbf{V}'(0)]\rangle dt \\ &= \frac{1}{N_d}\sum_{i=1}^{N_d}\int_0^\infty \langle \mathbf{v}_i(t)\cdot \mathbf{v}_i(0)\rangle dt \\ &+ 2\frac{N_d}{N'}\frac{m}{m'}\int_0^\infty \langle \mathbf{V}(t)\cdot \mathbf{V}(0)\rangle dt \\ &+ \left(-\frac{N_d}{N'}\frac{m}{m'}\right)^2\int_0^\infty \langle \mathbf{V}(t)\cdot \mathbf{V}(0)\rangle dt \\ &= D_d + \frac{N_d}{N'}\frac{m}{m'}\left(2 + \frac{N_d}{N'}\frac{m}{m'}\right)\mathcal{D}_d. \end{aligned} \tag{S6}$$

An example of the difference between self-diffusivity and the diffusivity computed in the laboratory reference frame is shown, for the F ions of $PbF_2$, in Fig. S3.

All the MSD obtained for this work are computed with the ANALISI code [1], whose results were also checked, in preliminary simulations, with the TRAVIS code [2, 3].

### B. Short-range Coulomb model

I investigated the role of long-range interactions on these size effects, by running the $\ell = 2$ and $\ell = 3$ calculations with a short-range version of the Coulomb interaction, namely the damped shifted force (DSF) model [4] as implemented in LAMMPS. Even if the specific values of $D$ change with respect to the long-range counterpart,

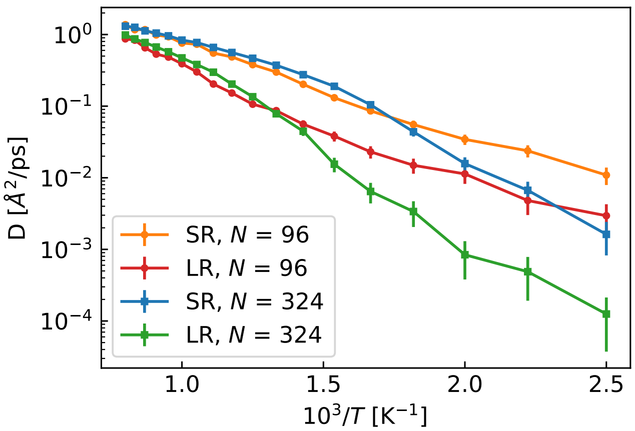


FIG. S4. Comparison between the short-range (SR) version of the Coulomb interaction, obtained through the DSF model with $r_c = a_{\mathrm{PbF}_2} = 6.056\,\mathrm{\AA}$ and $\alpha = 0.3\,\mathrm{\AA}$, and the long-range (LR) version, with the same cutoff $r_c$, but with Ewald's summations for Coulomb interactions. Even though the plots with SR seem to be shifted towards lower $T$, the striking difference between $N = 96$ and $N = 324$ is still observable.

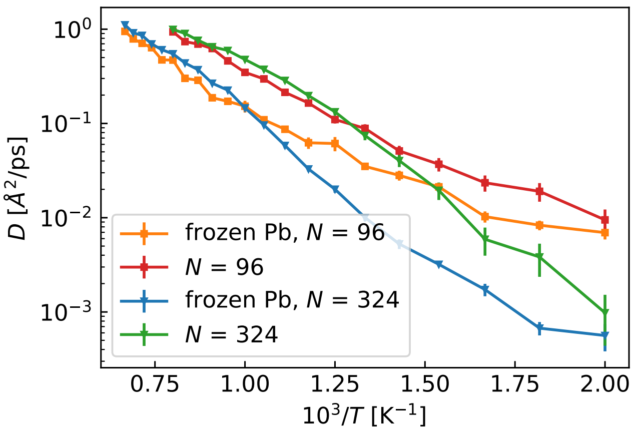


FIG. S5. Comparison between frozen-matrix (orange and blue) and standard (red and green) calculations. Even though the Arrhenius plots of the former appears shifted to higher temperatures with respect to the standard calculations, the same type of finite size effects is visible.

the qualitative difference between $N = 96$ (i.e. $\ell \leq 2$) and $N = 324$ (i.e. $\ell \geq 3$) still holds: with this potential, as well, the net change in $E_a$ by going from $T < T_c$ to $T > T_c$ is absent in $\ell = 2$ box.

### C. Frozen matrix calculation

In the frozen matrix simulation, the ions of the non-diffusing species are kept fixed in their equilibrium, high-symmetry positions and no evolution (i.e. no Verlet propagation) is applied to them. In this way, the diffusing ions move by feeling their mutual interaction and their interaction with fixed scatterers as in a pinball model [5]. Notice that in this way the position of the total centre of mass of the system is not conserved, and the frozen matrix simulation is *not* equivalent to a simulation with very heavy ions of the solid matrix which are nonetheless allowed to move. In particular, the reference frame in which the simulation is done coincides with the laboratory (and not the barycentric) reference frame.

The comparison between the diffusivity of F ions in the simulation run with frozen matrix and in the standard simulation is shown for $PbF_2$ in Fig. S5. It is evident that, even though the frozen matrix modifies the Arrhenius plots of $D$, in practice shifting the transition to the superionic phase towards larger temperatures, the finite-size effects observed in the standard simulations are still present.

### D. Size effects at low temperature

At low temperature, in fluorites, the diffusivity of the mobile anions is larger in smaller simulation cells. This is evidenced also by a direct inspection of the ionic positions along a trajectory, as reported in Fig. S6 for $PbF_2$ at $T = 600$ K. The related plot of the mean square displacement (MSD) of F ions is shown in Fig. S7. It has been argued [see Ref. 6, Sec. VI] that the use of log-log plots, for the MSD vs time, may identify possible caging effects whereby diffusing ions return back to their original position at intermediate timescales, and the diffusive behavior ($MSD \propto t$, i.e. unitary slope in log-log scale) is only observed for very long simulations. The log-log plot of Fig. S7 is shown in Fig. S8. The dotted black lines indicate the unitary-slope regimes. It would seem that a non-diffusive caging effect takes place for larger simulations at intermediate times. In practice, by carefully inspecting the simulations, I checked that, even if back-and-forth events—where a F ion returns to its initial position after some ps—are present, the lower diffusivity in larger systems is mainly due to a lower hopping rate than in smaller systems, and not to a true caging effect. A note: the reason why the unitary-slope regime is reached at larger times for larger simulation boxes is mainly due to the larger time at which the linear term $6Dt$ of the asymptotic behavior of the MSD becomes significant with respect to the intercept (here $\approx 1\,\mathrm{\AA}^2$, almost irrespective of the size). This happens at larger times for larger cell sizes due to the smaller diffusivity [7].

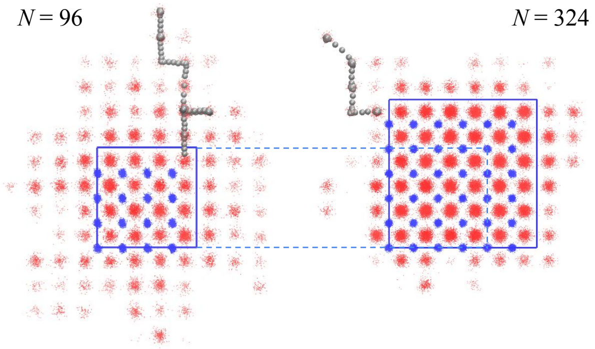


FIG. S6. Larger diffusion of F anion in smaller simulation box of $PbF_2$ at $T = 600$ K in the same time lap ($\approx 800$ ps). Unwrapped positions of Pb (blue) and F (red) ions along the trajectory, projected along the [001] direction, are displayed. The trajectory of one F ion is displayed in grey. The simulation box is highlighted (solid blue line).

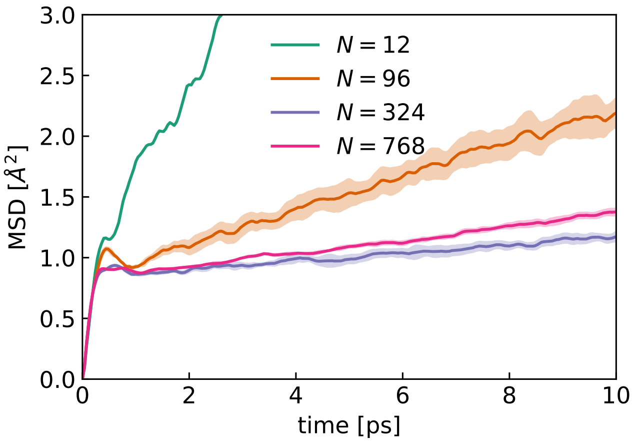


FIG. S7. Mean square displacement of F atoms in $PbF_2$ at $T = 600$ K and different cell sizes.

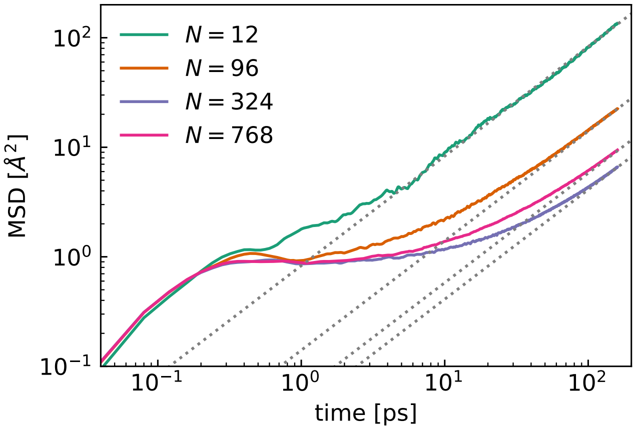


FIG. S8. Log-log plot of Fig. S7. Dotted lines indicate the slope = 1 behavior.

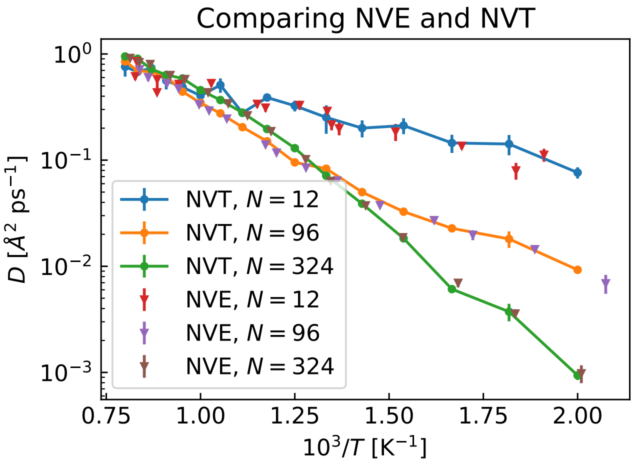


FIG. S9. Comparison of constant $NVT$ and $NVE$ ensembles in the calculation of the diffusion coefficient of F ions in $PbF_2$ at different cell sizes.

## S3. COMPARING $NVT$ AND $NVE$

I ran $NVE$ simulations to check that the values concerning the diffusivity of the mobile species, $D$, and the thermal conductivity, $\kappa$, do not depend on the specific thermodynamic ensemble, and that the stochastic velocity rescaling algorithm employed as thermostat in $NVT$ simulations is good also for extracting transport (dynamical) coefficients. Figures S9 and S10 show that, in typical simulations, the same results are practically obtained irrespective of the chosen ensemble. Obviously, the $NVT$ ensemble has the advantage, here, that it ensures a more precise control of the temperature with respect to previously equilibrated $NVE$ simulations. Furthermore, only within the $NVT$ ensemble can the isochoric heat capacity be computed.

## S4. THERMAL CONDUCTIVITY

### A. Details about the data analysis

As explained in Appendix A of the main manuscript, the calculation of the thermal conductivity is performed in frequency space, by investigating the low-frequency behavior of a properly defined power spectral density [see Eq. (A1)]. A recently developed *multivariate cepstral analysis* is applied to obtained an unbiased and consistent estimator of the thermal conductivity and of its uncertainty. I refer to Refs. [8, 9] for more details on the method. To have more statistics, I reshape the 3 time series (i.e. the $x$, $y$ and $z$ components) of the heat flux produced by LAMMPS in order to have more independent fluxes. Typically, I subdivide the timeseries into 8 blocks, for a total of 24 fluxes, which I used together in the statistical analysis. To select the number of cepstral coef-

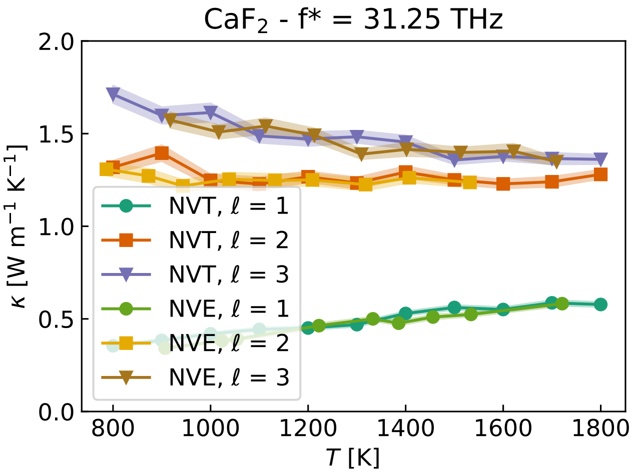


FIG. S10. Comparison of constant $NVT$ and $NVE$ ensembles in the calculation of the thermal conductivity $\kappa$ of $CaF_2$ at different cell sizes.

ficients to retain, I use the Akaike information criterion, according to its implementation in the SporTran code [10]. I also resample the trajectory so to focus the cepstral analysis on the low-frequency part of the heat flux power spectrum, i.e. up to a frequency $f^*$. Stable results are obtained with $f^* \approx 30$ THz for all the simulations.

### B. Virial part of heat flux in $UO_2$

Strictly speaking, for many-body potentials like the one used in $UO_2$, the virial part of the heat flux should be modified with respect to the form it assumes for two-body potentials [11]. In LAMMPS, the `compute centroid/stress/atom` command has been introduced to deal with 3- and 4-body interactions, for specific interatomic potentials [12, 13]. Unfortunately, the current implementation does not support models with long-range Coulombic interaction. Therefore, the results for the thermal conductivity of $UO_2$ employ the standard `compute stress/atom` command, which is formally correct only for two-body interactions. Still, I decided to retain these results since 1) the discrepancy between the two methods should be most important in low-dimensional systems (sheets, nanotubes, etc.) rather than in bulks [11]; 2) the EAM is just a correction to the other potentials and has a marginal role in heat flux; 3) I am interested in finite-size effects: should a deviation from the correct many-body virial part be relevant, it still does not affect, *a posteriori*, the general trend observed for fluorites, $UO_2$ included.

## S5. $B$-FACTOR

### A. Analytical derivation of $B$-factor correction

I start with the basic definition, i.e. the exponent

$$2W = \langle [\mathbf{q}\cdot\mathbf{u}]^2 \rangle \tag{S7}$$

of the Debye-Waller factor for the intensity (this is why the factor 2 is retained in the definition), $e^{-2W}$ [see Eq. (24.28) of Ref. 14]. Here $\mathbf{q}$ is the exchanged wave vector in the scattering, and $\mathbf{u}$ the displacement from equilibrium of the considered atom, which we consider at the lattice position $\mathbf{R} = 0$. For simplicity, I consider a monoatomic system with atomic mass $M$. In terms of normal modes, $\mathbf{u}$ can be written as [$\mathbf{k}$ is the wave vector, $s$ labels the polarization, and $\omega_s(\mathbf{k})$ is the related frequency]

$$\mathbf{u} = \frac{1}{\sqrt{N}} \sum_{\mathbf{k},s} \sqrt{\frac{\hbar}{2M\omega_s(\mathbf{k})}} (a_{\mathbf{k},s} + a^\dagger_{-\mathbf{k},s}) \boldsymbol{\epsilon}_s(\mathbf{k}) \tag{S8}$$

with the creation and annihilation operators satisfying

$$\begin{aligned} \langle a^\dagger_{\mathbf{k}',s'}\, a_{\mathbf{k},s}\rangle &= n_s(\mathbf{k})\, \delta_{\mathbf{k},\mathbf{k}'}\, \delta_{s,s'} \\ \langle a_{\mathbf{k},s}\, a^\dagger_{\mathbf{k}',s'}\rangle &= [1+n_s(\mathbf{k})]\, \delta_{\mathbf{k},\mathbf{k}'}\, \delta_{s,s'}, \end{aligned} \tag{S9}$$

$n_s(\mathbf{k}) \equiv 1/[\exp(\beta\hbar\omega_s(\mathbf{k})) - 1]$ being the Bose-Einstein distribution. Therefore:

$$\begin{aligned} 2W = \frac{\hbar}{2MN} \sum_{\mathbf{k},s} \sum_{\mathbf{k}',s'} \sqrt{\frac{1}{\omega_s(\mathbf{k})\omega_{s'}(\mathbf{k}')}} \times \\ [\mathbf{q}\cdot\boldsymbol{\epsilon}_s(\mathbf{k})][\mathbf{q}\cdot\boldsymbol{\epsilon}_{s'}(\mathbf{k}')] \underbrace{[\langle a_{\mathbf{k},s} a^\dagger_{-\mathbf{k}',s'}\rangle + \langle a^\dagger_{-\mathbf{k},s} a_{\mathbf{k}',s'}\rangle]}_{Q}. \end{aligned} \tag{S10}$$

I use the definition of the Bose-Einstein distribution in $Q$, and $\omega_s(\mathbf{k}) = \omega_s(-\mathbf{k})$:

$$\begin{aligned} Q &= [1+n_s(\mathbf{k})]\delta_{\mathbf{k},-\mathbf{k}'}\delta_{s,s'} + n_s(\mathbf{k})\delta_{\mathbf{k},-\mathbf{k}'}\delta_{s,s'} \\ &= \coth\left(\tfrac{1}{2}\beta\hbar\omega_s(\mathbf{k})\right) \delta_{\mathbf{k},-\mathbf{k}'}\delta_{s,s'}. \end{aligned} \tag{S11}$$

Finally, assuming $\boldsymbol{\epsilon}_s(\mathbf{k}) = \boldsymbol{\epsilon}_s(-\mathbf{k})$ (which is strictly valid for monoatomic sytems), I obtain, in the continuum limit,

$$2W = \frac{\hbar}{2\rho} \int \frac{d\mathbf{k}}{(2\pi)^3} \sum_s \frac{[\mathbf{q}\cdot\boldsymbol{\epsilon}_s(\mathbf{k})]^2}{\omega_s(\mathbf{k})} \coth\left(\tfrac{1}{2}\beta\hbar\omega_s(\mathbf{k})\right), \tag{S12}$$

where $\rho = MN/V$ is the mass density. This can be written easily for an isotropic system, where the result should not depend on the direction of $\mathbf{q}$. Since the polarizations can be taken orthogonal, so that $\boldsymbol{\epsilon}_s(\mathbf{k}) \cdot \boldsymbol{\epsilon}_{s'}(\mathbf{k}) = \delta_{s,s'}$, and since I can take $\mathbf{q}$ along any direction by isotropy,

by going to polar coordinates and integrating over the azimuthal angle, I obtain

$$2W = q^2 \frac{\hbar}{2\rho} \int \frac{k^2 dk \sin\theta d\theta}{(2\pi)^2} \sum_s \frac{\cos^2\theta}{\omega_s(\mathbf{k})} \coth\left(\tfrac{1}{2}\beta\hbar\omega_s(\mathbf{k})\right) = q^2 \frac{\hbar}{\rho} \int \frac{dk k^2}{(2\pi)^2} \underbrace{\frac{1}{3} \sum_s \frac{\coth\left(\frac{1}{2}\beta\hbar\omega_s(\mathbf{k})\right)}{\omega_s(\mathbf{k})}}_{\mathfrak{S}} \tag{S13}$$

By separating $t$ransverse and $l$ongitudinal modes, in the limit of low (acoustic) frequencies, $\mathfrak{S} \to 2/(\beta\hbar c^2 k^2)$, where

$$\frac{1}{c^2} = \frac{1}{3}\left[\frac{2}{c_t^2} + \frac{1}{c_l^2}\right] = \frac{\rho}{3}\left[\frac{2}{G} + \frac{1}{K + \frac{4}{3}G}\right] \equiv \frac{\rho}{K^{\rm eff}}, \tag{S14}$$

$c_t$ and $c_l$ are the transverse and longitudinal speeds of sound, $K$ and $G$ are the bulk and shear moduli, respectively, and where I used $\coth(x) \approx 1/x$ when $x$ is small.

Therefore, the finite-size correction to the infinite-size limit, due to the minimum finite frequency, is

$$\Delta 2W = \frac{q^2}{\beta\rho} \int_0^{\frac{2\pi}{a\ell}} \frac{dk k^2}{2\pi^2} \frac{1}{c^2 k^2} = q^2 \frac{1}{\beta\rho\pi c^2 a} \frac{1}{\ell} = q^2 \frac{1}{\beta\pi K^{\rm eff} a} \frac{1}{\ell} \tag{S15}$$

By comparison with Eq. (S7), which for an isotropic system becomes $2W = q^2\langle u^2\rangle/3$, this implies that the $B$-factor, defined by $B = 8\pi^2\langle u^2\rangle/3$, can be expressed as

$$B(\ell) = B(\infty) - \Delta B(\ell), \tag{S16}$$

where the finite-size correction is

$$\Delta B(l) = \frac{8\pi}{\beta K^{\rm eff} a} \frac{1}{\ell}. \tag{S17}$$

I checked this equation on a simple system (solid argon), as reported below, in Sec. S5.B. Notice that $\Delta B(l)$ does not depend on the mass $M$, in line with the fact that the asymptotic value of the mean square displacement is an equilibrium, time-independent property. In fact, I ran a set of simulations of $PbF_2$ where the mass of Pb was set to $m^*_{\rm Pb} = 4m_{\rm Pb}$, where $m_{\rm Pb}$ is the true mass of Pb. Figure S11 shows the MSD of Pb as a function of time, extracted from simulations at $T = 1000$ K and different sizes, run with the true Pb mass, $m_{\rm Pb}$, (olive, ocher, brown and grey) and $m^*_{\rm Pb}$ (teal, orange, violet, magenta). The initial behavior significantly differs between the two sets of simulations: for each size, the oscillations of the simulations run with $m^*$, have a frequency which is half (i.e. $\sqrt{m_{\rm Pb}/m^*_{\rm Pb}}$) that of the simulations $m_{\rm Pb}$. Nonetheless, the asymptotic values, and thus the $B$-factor, are independent of the mass of the ions.

I finally report the expression of the finite size effects within the Debye model, where [see Ref. 15, Eq. (7)]

$$B_{\rm D} = \frac{12\pi^2\hbar^4\beta_{\rm D}^3}{M} \int_0^{\omega_{\rm D}} \omega \coth(\tfrac{1}{2}\beta\hbar\omega) d\omega \tag{S18}$$

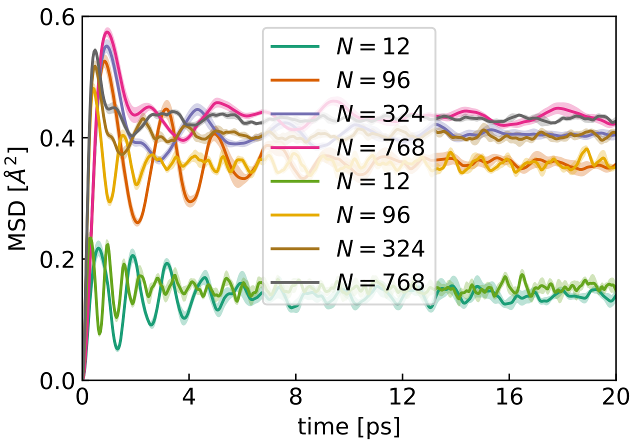


FIG. S11. MSD of Pb as a function of time, extracted from simulations at $T = 1000$ K and different sizes, run with the true Pb mass, $m_{\rm Pb}$, (olive, ocher, brown and grey) and $m^*_{\rm Pb}$ (teal, orange, violet, magenta).

where $1/\beta_{\rm D} = \hbar\omega_{\rm D}$, and the Debye angular frequency is defined by

$$\omega_{\rm D}^3 = \frac{6\pi^2 N}{V} c_{\rm D}^3 \tag{S19}$$

where the effective speed of sound in the Debye model is defined by

$$\frac{1}{c_{\rm D}^3} = \frac{1}{3}\left[\frac{2}{c_t^3} + \frac{1}{c_l^3}\right]. \tag{S20}$$

By expanding $\coth(\frac{1}{2}\beta\hbar\omega) \approx 2/(\beta\hbar\omega)$ and proceeding as before by integrating up to the minimum angular frequency $\omega_{\rm min} = 2\pi c_{\rm D}/(a\ell)$, I obtain the finite-size corrections to $B_D$:

$$\Delta B_{\rm D} = \frac{8\pi}{\beta K_{\rm D}^{\rm eff} a} \frac{1}{\ell} \tag{S21}$$

which is formally equivalent to Eq. (S17), even if, here, the effective elastic modulus is defined by

$$K_{\rm D}^{\rm eff} \equiv \left[\frac{2}{3}\sqrt{\frac{1}{G^3}} + \frac{1}{3}\sqrt{\frac{1}{(K + \frac{4}{3}G)^3}}\right]^{-2/3}. \tag{S22}$$

### B. Finite-size check for solid argon

I computed the $B$-factor for solid argon to check the validity of the behavior described. The density was fixed to 1.6451 g cm$^{-3}$, which is equivalent to a lattice constant $a$ = 5.4434 Å. The results are displayed in Fig. S12. The $1/\ell$ behavior of the finite-size effects is evident. The effective modulus $K^{\rm eff} \equiv 1/|m|$ obtained from the slope ranges from 1.31 to 1.19 GPa by increasing $T$. At the same density and $T = 76.8$ K, experimental values for

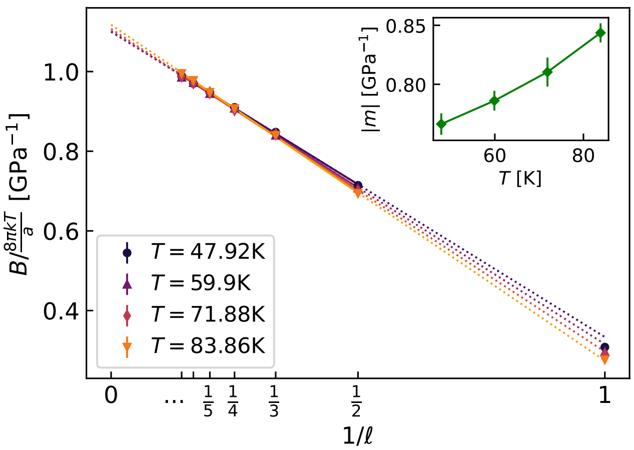


FIG. S12. Finite-size effects in the $B$-factor of Ar atoms at different temperatures. The lattice constant is fixed $a = 5.4434$ Å. The dotted lines are extrapolation. $\ell = 1$ is excluded from the fit.

$G = 1.0$ GPa and $K = 1.8$ GPa [16] give $K^{\text{eff}} = 1.29$ GPa and $K_{\text{D}}^{\text{eff}} = 1.17$ GPa, in good agreement with my simulations.

## S6. ROLE OF $F^-$ EMPTY SITES: HEAT CAPACITY

Figure S13 shows the isochoric specific heat capacity, $c_V$, of the defected lead fluorite system, as described in Appendix B of the main manuscript. The peak indicates a phase transition. I checked that this is not the transition to the liquid phase by direct inspection of the simulations, where Pb ions are always arranged as a crystalline matrix for all temperatures and sizes.

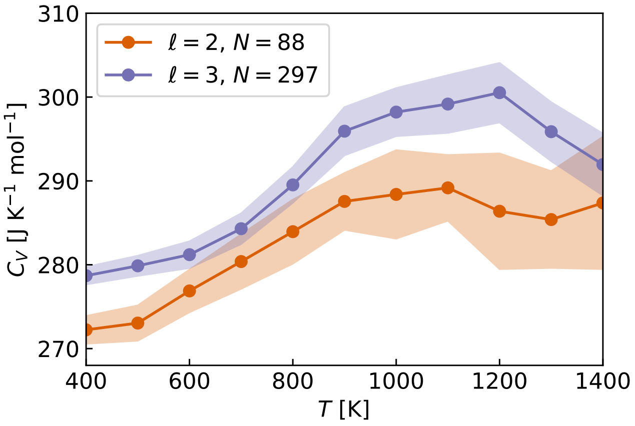


FIG. S13. Isochoric specific heat capacity, $c_V$, of the systems with defects, in J $K^{-1}$ per mole of $Pb_4F_7$.

## SUPPLEMENTARY REFERENCES

[1] R. Bertossa, "ANALISI: your swiss army knife of molecular dynamics analysis," `https://github.com/rikigigi/analisi` (2017–2022).
[2] M. Brehm and B. Kirchner, J. Chem. Inf. Model. **51**, 2007–2023 (2011).
[3] M. Brehm, M. Thomas, S. Gehrke, and B. Kirchner, The Journal of chemical physics **152**, 164105 (2020).
[4] C. J. Fennell and J. D. Gezelter, The Journal of chemical physics **124**, 234104 (2006).
[5] L. Kahle, A. Marcolongo, and N. Marzari, Physical Review Materials **2**, 065405 (2018).
[6] K. Funke, Progress in Solid State Chemistry **22**, 111 (1993).
[7] A straight line $y = mx + q$ with $q > 0$ in linear-linear plot becomes a unitary-slope line in the corresponding log-log plot only for $x$ such that $mx \gg q$.
[8] L. Ercole, A. Marcolongo, and S. Baroni, Sci. Rep. **7**, 15835 (2017), arXiv:1706.01381.
[9] R. Bertossa, F. Grasselli, L. Ercole, and S. Baroni, Phys. Rev. Lett. **122**, 255901 (2019).
[10] L. Ercole, R. Bertossa, S. Bisacchi, and S. Baroni, "SPORTRAN: a code to estimate transport coefficients from the cepstral analysis of (multi-variate) current time series," arXiv preprint arXiv:2202.11571, and `https://github.com/sissaschool/sportran` (2017–2022).
[11] Z. Fan, L. F. C. Pereira, H.-Q. Wang, J.-C. Zheng, D. Donadio, and A. Harju, Physical Review B **92**, 094301 (2015).
[12] P. Boone, H. Babaei, and C. E. Wilmer, Journal of chemical theory and computation **15**, 5579 (2019).
[13] D. Surblys, H. Matsubara, G. Kikugawa, and T. Ohara, Physical Review E **99**, 051301 (2019).
[14] N. W. Ashcroft and N. D. Mermin, *Solid state physics* (Holt, Rinehart and Winston, New York-London, 1976).
[15] C. Malica and A. Dal Corso, Acta Crystallographica Section A **75**, 624 (2019).
[16] G. Simmons, H. Wang, *et al.*, *Single crystal elastic constants and calculated aggregate properties* (Mass., MIt Press, 1971).
